# Supplementary material for: HoughCL: Finding Better Positive Pairs in Dense Self-supervised Learning
Source: arXiv:2111.10794 source file (2021-11-21)
Supplement: Supplementary file 1 [file additional_loss_spaces.tex]

%%%%%%%%%%%%%%%%%%%%%%%%%%%%%%%%%%%%%%%%%%%%%%%%%%%%%%%%%%%%%%%%%%%%%%%%%%%%%%%%
\subsection{Loss Surfaces for \data{PACS}}
\begin{figure}[H]
\centering
\captionsetup[subfigure]{aboveskip=0pt,belowskip=0pt}
\begin{subfigure}[b]{0.24\columnwidth}
    \includegraphics[width=\textwidth]{figures/all_loss_surfaces/PACS/TE0_env1_in_loss_plane.pdf}
    \caption{\textit{Cartoon} \scriptsize{(train)}}
\end{subfigure}
\begin{subfigure}[b]{0.24\columnwidth}
    \includegraphics[width=\textwidth]{figures/all_loss_surfaces/PACS/TE0_env2_in_loss_plane.pdf}
    \caption{\textit{Photo} \scriptsize{(train)}}
\end{subfigure}
\begin{subfigure}[b]{0.24\columnwidth}
    \includegraphics[width=\textwidth]{figures/all_loss_surfaces/PACS/TE0_env3_in_loss_plane.pdf}
    \caption{\textit{Sketch} \scriptsize{(train)}}
\end{subfigure}
\\
\begin{subfigure}[b]{0.18\columnwidth}
    \includegraphics[width=\textwidth]{figures/all_loss_surfaces/PACS/TE0_env1_out_loss_plane.pdf}
    \caption{\textit{Cartoon} \scriptsize{(valid)}}
\end{subfigure}
\begin{subfigure}[b]{0.18\columnwidth}
    \includegraphics[width=\textwidth]{figures/all_loss_surfaces/PACS/TE0_env2_out_loss_plane.pdf}
    \caption{\textit{Photo} \scriptsize{(valid)}}
\end{subfigure}
\begin{subfigure}[b]{0.18\columnwidth}
    \includegraphics[width=\textwidth]{figures/all_loss_surfaces/PACS/TE0_env3_out_loss_plane.pdf}
    \caption{\textit{Sketch} \scriptsize{(valid)}}
\end{subfigure}
\begin{subfigure}[b]{0.18\columnwidth}
    \includegraphics[width=\textwidth]{figures/all_loss_surfaces/PACS/TE0_env0_in_loss_plane.pdf}
    \caption{\textit{Art painting} \scriptsize{(test)}}
\end{subfigure}
\vspace{-0.5em}
\caption{\textbf{Visualization of loss surfaces for \data{PACS} when the target domain is \textit{Art painting}.}
}
\label{figure:add_loss_surface_PACS_Art painting}
\end{figure}
%%%%%%%%%%%%%%%%%%%%%%%%%%%%%%%%%%%%%%%%%%%%%%%%%%%%%%%%%%%%%%%%%%%%%%%%%%%%%%%%
\begin{figure}[H]
\centering
\captionsetup[subfigure]{aboveskip=0pt,belowskip=0pt}
\begin{subfigure}[b]{0.24\columnwidth}
    \includegraphics[width=\textwidth]{figures/all_loss_surfaces/PACS/TE1_env0_in_loss_plane.pdf}
    \caption{\textit{Art painting} \scriptsize{(train)}}
\end{subfigure}
\begin{subfigure}[b]{0.24\columnwidth}
    \includegraphics[width=\textwidth]{figures/all_loss_surfaces/PACS/TE1_env2_in_loss_plane.pdf}
    \caption{\textit{Photo} \scriptsize{(train)}}
\end{subfigure}
\begin{subfigure}[b]{0.24\columnwidth}
    \includegraphics[width=\textwidth]{figures/all_loss_surfaces/PACS/TE1_env3_in_loss_plane.pdf}
    \caption{\textit{Sketch} \scriptsize{(train)}}
\end{subfigure}
\\
\begin{subfigure}[b]{0.18\columnwidth}
    \includegraphics[width=\textwidth]{figures/all_loss_surfaces/PACS/TE1_env0_out_loss_plane.pdf}
    \caption{\textit{Art painting} \scriptsize{(valid)}}
\end{subfigure}
\begin{subfigure}[b]{0.18\columnwidth}
    \includegraphics[width=\textwidth]{figures/all_loss_surfaces/PACS/TE1_env2_out_loss_plane.pdf}
    \caption{\textit{Photo} \scriptsize{(valid)}}
\end{subfigure}
\begin{subfigure}[b]{0.18\columnwidth}
    \includegraphics[width=\textwidth]{figures/all_loss_surfaces/PACS/TE1_env3_out_loss_plane.pdf}
    \caption{\textit{Sketch} \scriptsize{(valid)}}
\end{subfigure}
\begin{subfigure}[b]{0.18\columnwidth}
    \includegraphics[width=\textwidth]{figures/all_loss_surfaces/PACS/TE1_env1_in_loss_plane.pdf}
    \caption{\textit{Cartoon} \scriptsize{(test)}}
\end{subfigure}
\vspace{-0.5em}
\caption{\textbf{Visualization of loss surfaces for \data{PACS} when the target domain is \textit{Cartoon}.}
}
\label{figure:add_loss_surface_PACS_Cartoon}
\end{figure}
%%%%%%%%%%%%%%%%%%%%%%%%%%%%%%%%%%%%%%%%%%%%%%%%%%%%%%%%%%%%%%%%%%%%%%%%%%%%%%%%
\begin{figure}[H]
\centering
\captionsetup[subfigure]{aboveskip=0pt,belowskip=0pt}
\begin{subfigure}[b]{0.24\columnwidth}
    \includegraphics[width=\textwidth]{figures/all_loss_surfaces/PACS/TE2_env0_in_loss_plane.pdf}
    \caption{\textit{Art painting} \scriptsize{(train)}}
\end{subfigure}
\begin{subfigure}[b]{0.24\columnwidth}
    \includegraphics[width=\textwidth]{figures/all_loss_surfaces/PACS/TE2_env1_in_loss_plane.pdf}
    \caption{\textit{Cartoon} \scriptsize{(train)}}
\end{subfigure}
\begin{subfigure}[b]{0.24\columnwidth}
    \includegraphics[width=\textwidth]{figures/all_loss_surfaces/PACS/TE2_env3_in_loss_plane.pdf}
    \caption{\textit{Sketch} \scriptsize{(train)}}
\end{subfigure}
\\
\begin{subfigure}[b]{0.18\columnwidth}
    \includegraphics[width=\textwidth]{figures/all_loss_surfaces/PACS/TE2_env0_out_loss_plane.pdf}
    \caption{\textit{Art painting} \scriptsize{(valid)}}
\end{subfigure}
\begin{subfigure}[b]{0.18\columnwidth}
    \includegraphics[width=\textwidth]{figures/all_loss_surfaces/PACS/TE2_env1_out_loss_plane.pdf}
    \caption{\textit{Cartoon} \scriptsize{(valid)}}
\end{subfigure}
\begin{subfigure}[b]{0.18\columnwidth}
    \includegraphics[width=\textwidth]{figures/all_loss_surfaces/PACS/TE2_env3_out_loss_plane.pdf}
    \caption{\textit{Sketch} \scriptsize{(valid)}}
\end{subfigure}
\begin{subfigure}[b]{0.18\columnwidth}
    \includegraphics[width=\textwidth]{figures/all_loss_surfaces/PACS/TE2_env2_in_loss_plane.pdf}
    \caption{\textit{Photo} \scriptsize{(test)}}
\end{subfigure}
\vspace{-0.5em}
\caption{\textbf{Visualization of loss surfaces for \data{PACS} when the target domain is \textit{Photo}.}
}
\label{figure:add_loss_surface_PACS_Photo}
\end{figure}
%%%%%%%%%%%%%%%%%%%%%%%%%%%%%%%%%%%%%%%%%%%%%%%%%%%%%%%%%%%%%%%%%%%%%%%%%%%%%%%%
\begin{figure}[H]
\centering
\captionsetup[subfigure]{aboveskip=0pt,belowskip=0pt}
\begin{subfigure}[b]{0.24\columnwidth}
    \includegraphics[width=\textwidth]{figures/all_loss_surfaces/PACS/TE3_env0_in_loss_plane.pdf}
    \caption{\textit{Art painting} \scriptsize{(train)}}
\end{subfigure}
\begin{subfigure}[b]{0.24\columnwidth}
    \includegraphics[width=\textwidth]{figures/all_loss_surfaces/PACS/TE3_env1_in_loss_plane.pdf}
    \caption{\textit{Cartoon} \scriptsize{(train)}}
\end{subfigure}
\begin{subfigure}[b]{0.24\columnwidth}
    \includegraphics[width=\textwidth]{figures/all_loss_surfaces/PACS/TE3_env2_in_loss_plane.pdf}
    \caption{\textit{Photo} \scriptsize{(train)}}
\end{subfigure}
\\
\begin{subfigure}[b]{0.18\columnwidth}
    \includegraphics[width=\textwidth]{figures/all_loss_surfaces/PACS/TE3_env0_out_loss_plane.pdf}
    \caption{\textit{Art painting} \scriptsize{(valid)}}
\end{subfigure}
\begin{subfigure}[b]{0.18\columnwidth}
    \includegraphics[width=\textwidth]{figures/all_loss_surfaces/PACS/TE3_env1_out_loss_plane.pdf}
    \caption{\textit{Cartoon} \scriptsize{(valid)}}
\end{subfigure}
\begin{subfigure}[b]{0.18\columnwidth}
    \includegraphics[width=\textwidth]{figures/all_loss_surfaces/PACS/TE3_env2_out_loss_plane.pdf}
    \caption{\textit{Photo} \scriptsize{(valid)}}
\end{subfigure}
\begin{subfigure}[b]{0.18\columnwidth}
    \includegraphics[width=\textwidth]{figures/all_loss_surfaces/PACS/TE3_env3_in_loss_plane.pdf}
    \caption{\textit{Sketch} \scriptsize{(test)}}
\end{subfigure}
\vspace{-0.5em}
\caption{\textbf{Visualization of loss surfaces for \data{PACS} when the target domain is \textit{Sketch}.}
}
\label{figure:add_loss_surface_PACS_Sketch}
\end{figure}
%%%%%%%%%%%%%%%%%%%%%%%%%%%%%%%%%%%%%%%%%%%%%%%%%%%%%%%%%%%%%%%%%%%%%%%%%%%%%%%%
%%%%%%%%%%%%%%%%%%%%%%%%%%%%%%%%%%%%%%%%%%%%%%%%%%%%%%%%%%%%%%%%%%%%%%%%%%%%%%%%
\subsection{Loss Surfaces for \data{VLCS}}
\begin{figure}[H]
\centering
\captionsetup[subfigure]{aboveskip=0pt,belowskip=0pt}
\begin{subfigure}[b]{0.24\columnwidth}
    \includegraphics[width=\textwidth]{figures/all_loss_surfaces/VLCS/TE0_env1_in_loss_plane.pdf}
    \caption{\textit{LabelMe} \scriptsize{(train)}}
\end{subfigure}
\begin{subfigure}[b]{0.24\columnwidth}
    \includegraphics[width=\textwidth]{figures/all_loss_surfaces/VLCS/TE0_env2_in_loss_plane.pdf}
    \caption{\textit{SUN09} \scriptsize{(train)}}
\end{subfigure}
\begin{subfigure}[b]{0.24\columnwidth}
    \includegraphics[width=\textwidth]{figures/all_loss_surfaces/VLCS/TE0_env3_in_loss_plane.pdf}
    \caption{\textit{VOC2007} \scriptsize{(train)}}
\end{subfigure}
\\
\begin{subfigure}[b]{0.18\columnwidth}
    \includegraphics[width=\textwidth]{figures/all_loss_surfaces/VLCS/TE0_env1_out_loss_plane.pdf}
    \caption{\textit{LabelMe} \scriptsize{(valid)}}
\end{subfigure}
\begin{subfigure}[b]{0.18\columnwidth}
    \includegraphics[width=\textwidth]{figures/all_loss_surfaces/VLCS/TE0_env2_out_loss_plane.pdf}
    \caption{\textit{SUN09} \scriptsize{(valid)}}
\end{subfigure}
\begin{subfigure}[b]{0.18\columnwidth}
    \includegraphics[width=\textwidth]{figures/all_loss_surfaces/VLCS/TE0_env3_out_loss_plane.pdf}
    \caption{\textit{VOC2007} \scriptsize{(valid)}}
\end{subfigure}
\begin{subfigure}[b]{0.18\columnwidth}
    \includegraphics[width=\textwidth]{figures/all_loss_surfaces/VLCS/TE0_env0_in_loss_plane.pdf}
    \caption{\textit{Caltech101} \scriptsize{(test)}}
\end{subfigure}
\vspace{-0.5em}
\caption{\textbf{Visualization of loss surfaces for \data{VLCS} when the target domain is \textit{Caltech101}.}
}
\label{figure:add_loss_surface_VLCS_Caltech101}
\end{figure}
%%%%%%%%%%%%%%%%%%%%%%%%%%%%%%%%%%%%%%%%%%%%%%%%%%%%%%%%%%%%%%%%%%%%%%%%%%%%%%%%
\begin{figure}[H]
\centering
\captionsetup[subfigure]{aboveskip=0pt,belowskip=0pt}
\begin{subfigure}[b]{0.24\columnwidth}
    \includegraphics[width=\textwidth]{figures/all_loss_surfaces/VLCS/TE1_env0_in_loss_plane.pdf}
    \caption{\textit{Caltech101} \scriptsize{(train)}}
\end{subfigure}
\begin{subfigure}[b]{0.24\columnwidth}
    \includegraphics[width=\textwidth]{figures/all_loss_surfaces/VLCS/TE1_env2_in_loss_plane.pdf}
    \caption{\textit{SUN09} \scriptsize{(train)}}
\end{subfigure}
\begin{subfigure}[b]{0.24\columnwidth}
    \includegraphics[width=\textwidth]{figures/all_loss_surfaces/VLCS/TE1_env3_in_loss_plane.pdf}
    \caption{\textit{VOC2007} \scriptsize{(train)}}
\end{subfigure}
\\
\begin{subfigure}[b]{0.18\columnwidth}
    \includegraphics[width=\textwidth]{figures/all_loss_surfaces/VLCS/TE1_env0_out_loss_plane.pdf}
    \caption{\textit{Caltech101} \scriptsize{(valid)}}
\end{subfigure}
\begin{subfigure}[b]{0.18\columnwidth}
    \includegraphics[width=\textwidth]{figures/all_loss_surfaces/VLCS/TE1_env2_out_loss_plane.pdf}
    \caption{\textit{SUN09} \scriptsize{(valid)}}
\end{subfigure}
\begin{subfigure}[b]{0.18\columnwidth}
    \includegraphics[width=\textwidth]{figures/all_loss_surfaces/VLCS/TE1_env3_out_loss_plane.pdf}
    \caption{\textit{VOC2007} \scriptsize{(valid)}}
\end{subfigure}
\begin{subfigure}[b]{0.18\columnwidth}
    \includegraphics[width=\textwidth]{figures/all_loss_surfaces/VLCS/TE1_env1_in_loss_plane.pdf}
    \caption{\textit{LabelMe} \scriptsize{(test)}}
\end{subfigure}
\vspace{-0.5em}
\caption{\textbf{Visualization of loss surfaces for \data{VLCS} when the target domain is \textit{LabelMe}.}
}
\label{figure:add_loss_surface_VLCS_LabelMe}
\end{figure}
%%%%%%%%%%%%%%%%%%%%%%%%%%%%%%%%%%%%%%%%%%%%%%%%%%%%%%%%%%%%%%%%%%%%%%%%%%%%%%%%
\begin{figure}[H]
\centering
\captionsetup[subfigure]{aboveskip=0pt,belowskip=0pt}
\begin{subfigure}[b]{0.24\columnwidth}
    \includegraphics[width=\textwidth]{figures/all_loss_surfaces/VLCS/TE2_env0_in_loss_plane.pdf}
    \caption{\textit{Caltech101} \scriptsize{(train)}}
\end{subfigure}
\begin{subfigure}[b]{0.24\columnwidth}
    \includegraphics[width=\textwidth]{figures/all_loss_surfaces/VLCS/TE2_env1_in_loss_plane.pdf}
    \caption{\textit{LabelMe} \scriptsize{(train)}}
\end{subfigure}
\begin{subfigure}[b]{0.24\columnwidth}
    \includegraphics[width=\textwidth]{figures/all_loss_surfaces/VLCS/TE2_env3_in_loss_plane.pdf}
    \caption{\textit{VOC2007} \scriptsize{(train)}}
\end{subfigure}
\\
\begin{subfigure}[b]{0.18\columnwidth}
    \includegraphics[width=\textwidth]{figures/all_loss_surfaces/VLCS/TE2_env0_out_loss_plane.pdf}
    \caption{\textit{Caltech101} \scriptsize{(valid)}}
\end{subfigure}
\begin{subfigure}[b]{0.18\columnwidth}
    \includegraphics[width=\textwidth]{figures/all_loss_surfaces/VLCS/TE2_env1_out_loss_plane.pdf}
    \caption{\textit{LabelMe} \scriptsize{(valid)}}
\end{subfigure}
\begin{subfigure}[b]{0.18\columnwidth}
    \includegraphics[width=\textwidth]{figures/all_loss_surfaces/VLCS/TE2_env3_out_loss_plane.pdf}
    \caption{\textit{VOC2007} \scriptsize{(valid)}}
\end{subfigure}
\begin{subfigure}[b]{0.18\columnwidth}
    \includegraphics[width=\textwidth]{figures/all_loss_surfaces/VLCS/TE2_env2_in_loss_plane.pdf}
    \caption{\textit{SUN09} \scriptsize{(test)}}
\end{subfigure}
\vspace{-0.5em}
\caption{\textbf{Visualization of loss surfaces for \data{VLCS} when the target domain is \textit{SUN09}.}
}
\label{figure:add_loss_surface_VLCS_SUN09}
\end{figure}
%%%%%%%%%%%%%%%%%%%%%%%%%%%%%%%%%%%%%%%%%%%%%%%%%%%%%%%%%%%%%%%%%%%%%%%%%%%%%%%%
\begin{figure}[H]
\centering
\captionsetup[subfigure]{aboveskip=0pt,belowskip=0pt}
\begin{subfigure}[b]{0.24\columnwidth}
    \includegraphics[width=\textwidth]{figures/all_loss_surfaces/VLCS/TE3_env0_in_loss_plane.pdf}
    \caption{\textit{Caltech101} \scriptsize{(train)}}
\end{subfigure}
\begin{subfigure}[b]{0.24\columnwidth}
    \includegraphics[width=\textwidth]{figures/all_loss_surfaces/VLCS/TE3_env1_in_loss_plane.pdf}
    \caption{\textit{LabelMe} \scriptsize{(train)}}
\end{subfigure}
\begin{subfigure}[b]{0.24\columnwidth}
    \includegraphics[width=\textwidth]{figures/all_loss_surfaces/VLCS/TE3_env2_in_loss_plane.pdf}
    \caption{\textit{SUN09} \scriptsize{(train)}}
\end{subfigure}
\\
\begin{subfigure}[b]{0.18\columnwidth}
    \includegraphics[width=\textwidth]{figures/all_loss_surfaces/VLCS/TE3_env0_out_loss_plane.pdf}
    \caption{\textit{Caltech101} \scriptsize{(valid)}}
\end{subfigure}
\begin{subfigure}[b]{0.18\columnwidth}
    \includegraphics[width=\textwidth]{figures/all_loss_surfaces/VLCS/TE3_env1_out_loss_plane.pdf}
    \caption{\textit{LabelMe} \scriptsize{(valid)}}
\end{subfigure}
\begin{subfigure}[b]{0.18\columnwidth}
    \includegraphics[width=\textwidth]{figures/all_loss_surfaces/VLCS/TE3_env2_out_loss_plane.pdf}
    \caption{\textit{SUN09} \scriptsize{(valid)}}
\end{subfigure}
\begin{subfigure}[b]{0.18\columnwidth}
    \includegraphics[width=\textwidth]{figures/all_loss_surfaces/VLCS/TE3_env3_in_loss_plane.pdf}
    \caption{\textit{VOC2007} \scriptsize{(test)}}
\end{subfigure}
\vspace{-0.5em}
\caption{\textbf{Visualization of loss surfaces for \data{VLCS} when the target domain is \textit{VOC2007}.}
}
\label{figure:add_loss_surface_VLCS_VOC2007}
\end{figure}
%%%%%%%%%%%%%%%%%%%%%%%%%%%%%%%%%%%%%%%%%%%%%%%%%%%%%%%%%%%%%%%%%%%%%%%%%%%%%%%%
%%%%%%%%%%%%%%%%%%%%%%%%%%%%%%%%%%%%%%%%%%%%%%%%%%%%%%%%%%%%%%%%%%%%%%%%%%%%%%%%
\subsection{Loss Surfaces for \data{OfficeHome}}
\begin{figure}[H]
\centering
\captionsetup[subfigure]{aboveskip=0pt,belowskip=0pt}
\begin{subfigure}[b]{0.24\columnwidth}
    \includegraphics[width=\textwidth]{figures/all_loss_surfaces/OfficeHome/TE0_env1_in_loss_plane.pdf}
    \caption{\textit{Clipart} \scriptsize{(train)}}
\end{subfigure}
\begin{subfigure}[b]{0.24\columnwidth}
    \includegraphics[width=\textwidth]{figures/all_loss_surfaces/OfficeHome/TE0_env2_in_loss_plane.pdf}
    \caption{\textit{Product} \scriptsize{(train)}}
\end{subfigure}
\begin{subfigure}[b]{0.24\columnwidth}
    \includegraphics[width=\textwidth]{figures/all_loss_surfaces/OfficeHome/TE0_env3_in_loss_plane.pdf}
    \caption{\textit{Real world} \scriptsize{(train)}}
\end{subfigure}
\\
\begin{subfigure}[b]{0.18\columnwidth}
    \includegraphics[width=\textwidth]{figures/all_loss_surfaces/OfficeHome/TE0_env1_out_loss_plane.pdf}
    \caption{\textit{Clipart} \scriptsize{(valid)}}
\end{subfigure}
\begin{subfigure}[b]{0.18\columnwidth}
    \includegraphics[width=\textwidth]{figures/all_loss_surfaces/OfficeHome/TE0_env2_out_loss_plane.pdf}
    \caption{\textit{Product} \scriptsize{(valid)}}
\end{subfigure}
\begin{subfigure}[b]{0.18\columnwidth}
    \includegraphics[width=\textwidth]{figures/all_loss_surfaces/OfficeHome/TE0_env3_out_loss_plane.pdf}
    \caption{\textit{Real world} \scriptsize{(valid)}}
\end{subfigure}
\begin{subfigure}[b]{0.18\columnwidth}
    \includegraphics[width=\textwidth]{figures/all_loss_surfaces/OfficeHome/TE0_env0_in_loss_plane.pdf}
    \caption{\textit{Art} \scriptsize{(test)}}
\end{subfigure}
\vspace{-0.5em}
\caption{\textbf{Visualization of loss surfaces for \data{OfficeHome} when the target domain is \textit{Art}.}
}
\label{figure:add_loss_surface_OfficeHome_Art}
\end{figure}
%%%%%%%%%%%%%%%%%%%%%%%%%%%%%%%%%%%%%%%%%%%%%%%%%%%%%%%%%%%%%%%%%%%%%%%%%%%%%%%%
\begin{figure}[H]
\centering
\captionsetup[subfigure]{aboveskip=0pt,belowskip=0pt}
\begin{subfigure}[b]{0.24\columnwidth}
    \includegraphics[width=\textwidth]{figures/all_loss_surfaces/OfficeHome/TE1_env0_in_loss_plane.pdf}
    \caption{\textit{Art} \scriptsize{(train)}}
\end{subfigure}
\begin{subfigure}[b]{0.24\columnwidth}
    \includegraphics[width=\textwidth]{figures/all_loss_surfaces/OfficeHome/TE1_env2_in_loss_plane.pdf}
    \caption{\textit{Product} \scriptsize{(train)}}
\end{subfigure}
\begin{subfigure}[b]{0.24\columnwidth}
    \includegraphics[width=\textwidth]{figures/all_loss_surfaces/OfficeHome/TE1_env3_in_loss_plane.pdf}
    \caption{\textit{Real world} \scriptsize{(train)}}
\end{subfigure}
\\
\begin{subfigure}[b]{0.18\columnwidth}
    \includegraphics[width=\textwidth]{figures/all_loss_surfaces/OfficeHome/TE1_env0_out_loss_plane.pdf}
    \caption{\textit{Art} \scriptsize{(valid)}}
\end{subfigure}
\begin{subfigure}[b]{0.18\columnwidth}
    \includegraphics[width=\textwidth]{figures/all_loss_surfaces/OfficeHome/TE1_env2_out_loss_plane.pdf}
    \caption{\textit{Product} \scriptsize{(valid)}}
\end{subfigure}
\begin{subfigure}[b]{0.18\columnwidth}
    \includegraphics[width=\textwidth]{figures/all_loss_surfaces/OfficeHome/TE1_env3_out_loss_plane.pdf}
    \caption{\textit{Real world} \scriptsize{(valid)}}
\end{subfigure}
\begin{subfigure}[b]{0.18\columnwidth}
    \includegraphics[width=\textwidth]{figures/all_loss_surfaces/OfficeHome/TE1_env1_in_loss_plane.pdf}
    \caption{\textit{Clipart} \scriptsize{(test)}}
\end{subfigure}
\vspace{-0.5em}
\caption{\textbf{Visualization of loss surfaces for \data{OfficeHome} when the target domain is \textit{Clipart}.}
}
\label{figure:add_loss_surface_OfficeHome_Clipart}
\end{figure}
%%%%%%%%%%%%%%%%%%%%%%%%%%%%%%%%%%%%%%%%%%%%%%%%%%%%%%%%%%%%%%%%%%%%%%%%%%%%%%%%
\begin{figure}[H]
\centering
\captionsetup[subfigure]{aboveskip=0pt,belowskip=0pt}
\begin{subfigure}[b]{0.24\columnwidth}
    \includegraphics[width=\textwidth]{figures/all_loss_surfaces/OfficeHome/TE2_env0_in_loss_plane.pdf}
    \caption{\textit{Art} \scriptsize{(train)}}
\end{subfigure}
\begin{subfigure}[b]{0.24\columnwidth}
    \includegraphics[width=\textwidth]{figures/all_loss_surfaces/OfficeHome/TE2_env1_in_loss_plane.pdf}
    \caption{\textit{Clipart} \scriptsize{(train)}}
\end{subfigure}
\begin{subfigure}[b]{0.24\columnwidth}
    \includegraphics[width=\textwidth]{figures/all_loss_surfaces/OfficeHome/TE2_env3_in_loss_plane.pdf}
    \caption{\textit{Real world} \scriptsize{(train)}}
\end{subfigure}
\\
\begin{subfigure}[b]{0.18\columnwidth}
    \includegraphics[width=\textwidth]{figures/all_loss_surfaces/OfficeHome/TE2_env0_out_loss_plane.pdf}
    \caption{\textit{Art} \scriptsize{(valid)}}
\end{subfigure}
\begin{subfigure}[b]{0.18\columnwidth}
    \includegraphics[width=\textwidth]{figures/all_loss_surfaces/OfficeHome/TE2_env1_out_loss_plane.pdf}
    \caption{\textit{Clipart} \scriptsize{(valid)}}
\end{subfigure}
\begin{subfigure}[b]{0.18\columnwidth}
    \includegraphics[width=\textwidth]{figures/all_loss_surfaces/OfficeHome/TE2_env3_out_loss_plane.pdf}
    \caption{\textit{Real world} \scriptsize{(valid)}}
\end{subfigure}
\begin{subfigure}[b]{0.18\columnwidth}
    \includegraphics[width=\textwidth]{figures/all_loss_surfaces/OfficeHome/TE2_env2_in_loss_plane.pdf}
    \caption{\textit{Product} \scriptsize{(test)}}
\end{subfigure}
\vspace{-0.5em}
\caption{\textbf{Visualization of loss surfaces for \data{OfficeHome} when the target domain is \textit{Product}.}
}
\label{figure:add_loss_surface_OfficeHome_Product}
\end{figure}
%%%%%%%%%%%%%%%%%%%%%%%%%%%%%%%%%%%%%%%%%%%%%%%%%%%%%%%%%%%%%%%%%%%%%%%%%%%%%%%%
\begin{figure}[H]
\centering
\captionsetup[subfigure]{aboveskip=0pt,belowskip=0pt}
\begin{subfigure}[b]{0.24\columnwidth}
    \includegraphics[width=\textwidth]{figures/all_loss_surfaces/OfficeHome/TE3_env0_in_loss_plane.pdf}
    \caption{\textit{Art} \scriptsize{(train)}}
\end{subfigure}
\begin{subfigure}[b]{0.24\columnwidth}
    \includegraphics[width=\textwidth]{figures/all_loss_surfaces/OfficeHome/TE3_env1_in_loss_plane.pdf}
    \caption{\textit{Clipart} \scriptsize{(train)}}
\end{subfigure}
\begin{subfigure}[b]{0.24\columnwidth}
    \includegraphics[width=\textwidth]{figures/all_loss_surfaces/OfficeHome/TE3_env2_in_loss_plane.pdf}
    \caption{\textit{Product} \scriptsize{(train)}}
\end{subfigure}
\\
\begin{subfigure}[b]{0.18\columnwidth}
    \includegraphics[width=\textwidth]{figures/all_loss_surfaces/OfficeHome/TE3_env0_out_loss_plane.pdf}
    \caption{\textit{Art} \scriptsize{(valid)}}
\end{subfigure}
\begin{subfigure}[b]{0.18\columnwidth}
    \includegraphics[width=\textwidth]{figures/all_loss_surfaces/OfficeHome/TE3_env1_out_loss_plane.pdf}
    \caption{\textit{Clipart} \scriptsize{(valid)}}
\end{subfigure}
\begin{subfigure}[b]{0.18\columnwidth}
    \includegraphics[width=\textwidth]{figures/all_loss_surfaces/OfficeHome/TE3_env2_out_loss_plane.pdf}
    \caption{\textit{Product} \scriptsize{(valid)}}
\end{subfigure}
\begin{subfigure}[b]{0.18\columnwidth}
    \includegraphics[width=\textwidth]{figures/all_loss_surfaces/OfficeHome/TE3_env3_in_loss_plane.pdf}
    \caption{\textit{Real world} \scriptsize{(test)}}
\end{subfigure}
\vspace{-0.5em}
\caption{\textbf{Visualization of loss surfaces for \data{OfficeHome} when the target domain is \textit{Real world}.}
}
\label{figure:add_loss_surface_OfficeHome_Real world}
\end{figure}
%%%%%%%%%%%%%%%%%%%%%%%%%%%%%%%%%%%%%%%%%%%%%%%%%%%%%%%%%%%%%%%%%%%%%%%%%%%%%%%%
%%%%%%%%%%%%%%%%%%%%%%%%%%%%%%%%%%%%%%%%%%%%%%%%%%%%%%%%%%%%%%%%%%%%%%%%%%%%%%%%
\subsection{Loss Surfaces for \data{TerraIncognita}}
\begin{figure}[H]
\centering
\captionsetup[subfigure]{aboveskip=0pt,belowskip=0pt}
\begin{subfigure}[b]{0.24\columnwidth}
    \includegraphics[width=\textwidth]{figures/all_loss_surfaces/TerraIncognita/TE0_env1_in_loss_plane.pdf}
    \caption{\textit{Location38} \scriptsize{(train)}}
\end{subfigure}
\begin{subfigure}[b]{0.24\columnwidth}
    \includegraphics[width=\textwidth]{figures/all_loss_surfaces/TerraIncognita/TE0_env2_in_loss_plane.pdf}
    \caption{\textit{Location43} \scriptsize{(train)}}
\end{subfigure}
\begin{subfigure}[b]{0.24\columnwidth}
    \includegraphics[width=\textwidth]{figures/all_loss_surfaces/TerraIncognita/TE0_env3_in_loss_plane.pdf}
    \caption{\textit{Location46} \scriptsize{(train)}}
\end{subfigure}
\\
\begin{subfigure}[b]{0.18\columnwidth}
    \includegraphics[width=\textwidth]{figures/all_loss_surfaces/TerraIncognita/TE0_env1_out_loss_plane.pdf}
    \caption{\textit{Location38} \scriptsize{(valid)}}
\end{subfigure}
\begin{subfigure}[b]{0.18\columnwidth}
    \includegraphics[width=\textwidth]{figures/all_loss_surfaces/TerraIncognita/TE0_env2_out_loss_plane.pdf}
    \caption{\textit{Location43} \scriptsize{(valid)}}
\end{subfigure}
\begin{subfigure}[b]{0.18\columnwidth}
    \includegraphics[width=\textwidth]{figures/all_loss_surfaces/TerraIncognita/TE0_env3_out_loss_plane.pdf}
    \caption{\textit{Location46} \scriptsize{(valid)}}
\end{subfigure}
\begin{subfigure}[b]{0.18\columnwidth}
    \includegraphics[width=\textwidth]{figures/all_loss_surfaces/TerraIncognita/TE0_env0_in_loss_plane.pdf}
    \caption{\textit{Location100} \scriptsize{(test)}}
\end{subfigure}
\vspace{-0.5em}
\caption{\textbf{Visualization of loss surfaces for \data{TerraIncognita} when the target domain is \textit{Location100}.}
}
\label{figure:add_loss_surface_TerraIncognita_Location100}
\end{figure}
%%%%%%%%%%%%%%%%%%%%%%%%%%%%%%%%%%%%%%%%%%%%%%%%%%%%%%%%%%%%%%%%%%%%%%%%%%%%%%%%
\begin{figure}[H]
\centering
\captionsetup[subfigure]{aboveskip=0pt,belowskip=0pt}
\begin{subfigure}[b]{0.24\columnwidth}
    \includegraphics[width=\textwidth]{figures/all_loss_surfaces/TerraIncognita/TE1_env0_in_loss_plane.pdf}
    \caption{\textit{Location100} \scriptsize{(train)}}
\end{subfigure}
\begin{subfigure}[b]{0.24\columnwidth}
    \includegraphics[width=\textwidth]{figures/all_loss_surfaces/TerraIncognita/TE1_env2_in_loss_plane.pdf}
    \caption{\textit{Location43} \scriptsize{(train)}}
\end{subfigure}
\begin{subfigure}[b]{0.24\columnwidth}
    \includegraphics[width=\textwidth]{figures/all_loss_surfaces/TerraIncognita/TE1_env3_in_loss_plane.pdf}
    \caption{\textit{Location46} \scriptsize{(train)}}
\end{subfigure}
\\
\begin{subfigure}[b]{0.18\columnwidth}
    \includegraphics[width=\textwidth]{figures/all_loss_surfaces/TerraIncognita/TE1_env0_out_loss_plane.pdf}
    \caption{\textit{Location100} \scriptsize{(valid)}}
\end{subfigure}
\begin{subfigure}[b]{0.18\columnwidth}
    \includegraphics[width=\textwidth]{figures/all_loss_surfaces/TerraIncognita/TE1_env2_out_loss_plane.pdf}
    \caption{\textit{Location43} \scriptsize{(valid)}}
\end{subfigure}
\begin{subfigure}[b]{0.18\columnwidth}
    \includegraphics[width=\textwidth]{figures/all_loss_surfaces/TerraIncognita/TE1_env3_out_loss_plane.pdf}
    \caption{\textit{Location46} \scriptsize{(valid)}}
\end{subfigure}
\begin{subfigure}[b]{0.18\columnwidth}
    \includegraphics[width=\textwidth]{figures/all_loss_surfaces/TerraIncognita/TE1_env1_in_loss_plane.pdf}
    \caption{\textit{Location38} \scriptsize{(test)}}
\end{subfigure}
\vspace{-0.5em}
\caption{\textbf{Visualization of loss surfaces for \data{TerraIncognita} when the target domain is \textit{Location38}.}
}
\label{figure:add_loss_surface_TerraIncognita_Location38}
\end{figure}
%%%%%%%%%%%%%%%%%%%%%%%%%%%%%%%%%%%%%%%%%%%%%%%%%%%%%%%%%%%%%%%%%%%%%%%%%%%%%%%%
\begin{figure}[H]
\centering
\captionsetup[subfigure]{aboveskip=0pt,belowskip=0pt}
\begin{subfigure}[b]{0.24\columnwidth}
    \includegraphics[width=\textwidth]{figures/all_loss_surfaces/TerraIncognita/TE2_env0_in_loss_plane.pdf}
    \caption{\textit{Location100} \scriptsize{(train)}}
\end{subfigure}
\begin{subfigure}[b]{0.24\columnwidth}
    \includegraphics[width=\textwidth]{figures/all_loss_surfaces/TerraIncognita/TE2_env1_in_loss_plane.pdf}
    \caption{\textit{Location38} \scriptsize{(train)}}
\end{subfigure}
\begin{subfigure}[b]{0.24\columnwidth}
    \includegraphics[width=\textwidth]{figures/all_loss_surfaces/TerraIncognita/TE2_env3_in_loss_plane.pdf}
    \caption{\textit{Location46} \scriptsize{(train)}}
\end{subfigure}
\\
\begin{subfigure}[b]{0.18\columnwidth}
    \includegraphics[width=\textwidth]{figures/all_loss_surfaces/TerraIncognita/TE2_env0_out_loss_plane.pdf}
    \caption{\textit{Location100} \scriptsize{(valid)}}
\end{subfigure}
\begin{subfigure}[b]{0.18\columnwidth}
    \includegraphics[width=\textwidth]{figures/all_loss_surfaces/TerraIncognita/TE2_env1_out_loss_plane.pdf}
    \caption{\textit{Location38} \scriptsize{(valid)}}
\end{subfigure}
\begin{subfigure}[b]{0.18\columnwidth}
    \includegraphics[width=\textwidth]{figures/all_loss_surfaces/TerraIncognita/TE2_env3_out_loss_plane.pdf}
    \caption{\textit{Location46} \scriptsize{(valid)}}
\end{subfigure}
\begin{subfigure}[b]{0.18\columnwidth}
    \includegraphics[width=\textwidth]{figures/all_loss_surfaces/TerraIncognita/TE2_env2_in_loss_plane.pdf}
    \caption{\textit{Location43} \scriptsize{(test)}}
\end{subfigure}
\vspace{-0.5em}
\caption{\textbf{Visualization of loss surfaces for \data{TerraIncognita} when the target domain is \textit{Location43}.}
}
\label{figure:add_loss_surface_TerraIncognita_Location43}
\end{figure}
%%%%%%%%%%%%%%%%%%%%%%%%%%%%%%%%%%%%%%%%%%%%%%%%%%%%%%%%%%%%%%%%%%%%%%%%%%%%%%%%
\begin{figure}[H]
\centering
\captionsetup[subfigure]{aboveskip=0pt,belowskip=0pt}
\begin{subfigure}[b]{0.24\columnwidth}
    \includegraphics[width=\textwidth]{figures/all_loss_surfaces/TerraIncognita/TE3_env0_in_loss_plane.pdf}
    \caption{\textit{Location100} \scriptsize{(train)}}
\end{subfigure}
\begin{subfigure}[b]{0.24\columnwidth}
    \includegraphics[width=\textwidth]{figures/all_loss_surfaces/TerraIncognita/TE3_env1_in_loss_plane.pdf}
    \caption{\textit{Location38} \scriptsize{(train)}}
\end{subfigure}
\begin{subfigure}[b]{0.24\columnwidth}
    \includegraphics[width=\textwidth]{figures/all_loss_surfaces/TerraIncognita/TE3_env2_in_loss_plane.pdf}
    \caption{\textit{Location43} \scriptsize{(train)}}
\end{subfigure}
\\
\begin{subfigure}[b]{0.18\columnwidth}
    \includegraphics[width=\textwidth]{figures/all_loss_surfaces/TerraIncognita/TE3_env0_out_loss_plane.pdf}
    \caption{\textit{Location100} \scriptsize{(valid)}}
\end{subfigure}
\begin{subfigure}[b]{0.18\columnwidth}
    \includegraphics[width=\textwidth]{figures/all_loss_surfaces/TerraIncognita/TE3_env1_out_loss_plane.pdf}
    \caption{\textit{Location38} \scriptsize{(valid)}}
\end{subfigure}
\begin{subfigure}[b]{0.18\columnwidth}
    \includegraphics[width=\textwidth]{figures/all_loss_surfaces/TerraIncognita/TE3_env2_out_loss_plane.pdf}
    \caption{\textit{Location43} \scriptsize{(valid)}}
\end{subfigure}
\begin{subfigure}[b]{0.18\columnwidth}
    \includegraphics[width=\textwidth]{figures/all_loss_surfaces/TerraIncognita/TE3_env3_in_loss_plane.pdf}
    \caption{\textit{Location46} \scriptsize{(test)}}
\end{subfigure}
\vspace{-0.5em}
\caption{\textbf{Visualization of loss surfaces for \data{TerraIncognita} when the target domain is \textit{Location46}.}
}
\label{figure:add_loss_surface_TerraIncognita_Location46}
\end{figure}
%%%%%%%%%%%%%%%%%%%%%%%%%%%%%%%%%%%%%%%%%%%%%%%%%%%%%%%%%%%%%%%%%%%%%%%%%%%%%%%%
%%%%%%%%%%%%%%%%%%%%%%%%%%%%%%%%%%%%%%%%%%%%%%%%%%%%%%%%%%%%%%%%%%%%%%%%%%%%%%%%
\subsection{Loss Surfaces for \data{DomainNet}}
\begin{figure}[H]
\centering
\captionsetup[subfigure]{aboveskip=0pt,belowskip=0pt}
\begin{subfigure}[b]{0.19\columnwidth}
    \includegraphics[width=\textwidth]{figures/all_loss_surfaces/DomainNet/TE0_env1_in_loss_plane.pdf}
    \caption{\textit{Infographic} \scriptsize{(train)}}
\end{subfigure}
\begin{subfigure}[b]{0.19\columnwidth}
    \includegraphics[width=\textwidth]{figures/all_loss_surfaces/DomainNet/TE0_env2_in_loss_plane.pdf}
    \caption{\textit{Painting} \scriptsize{(train)}}
\end{subfigure}
\begin{subfigure}[b]{0.19\columnwidth}
    \includegraphics[width=\textwidth]{figures/all_loss_surfaces/DomainNet/TE0_env3_in_loss_plane.pdf}
    \caption{\textit{Quickdraw} \scriptsize{(train)}}
\end{subfigure}
\begin{subfigure}[b]{0.19\columnwidth}
    \includegraphics[width=\textwidth]{figures/all_loss_surfaces/DomainNet/TE0_env4_in_loss_plane.pdf}
    \caption{\textit{Real} \scriptsize{(train)}}
\end{subfigure}
\begin{subfigure}[b]{0.19\columnwidth}
    \includegraphics[width=\textwidth]{figures/all_loss_surfaces/DomainNet/TE0_env5_in_loss_plane.pdf}
    \caption{\textit{Sketch} \scriptsize{(train)}}
\end{subfigure}
\\
\begin{subfigure}[b]{0.16\columnwidth}
    \includegraphics[width=\textwidth]{figures/all_loss_surfaces/DomainNet/TE0_env1_out_loss_plane.pdf}
    \caption{\textit{Infographic} \scriptsize{(valid)}}
\end{subfigure}
\begin{subfigure}[b]{0.16\columnwidth}
    \includegraphics[width=\textwidth]{figures/all_loss_surfaces/DomainNet/TE0_env2_out_loss_plane.pdf}
    \caption{\textit{Painting} \scriptsize{(valid)}}
\end{subfigure}
\begin{subfigure}[b]{0.16\columnwidth}
    \includegraphics[width=\textwidth]{figures/all_loss_surfaces/DomainNet/TE0_env3_out_loss_plane.pdf}
    \caption{\textit{Quickdraw} \scriptsize{(valid)}}
\end{subfigure}
\begin{subfigure}[b]{0.16\columnwidth}
    \includegraphics[width=\textwidth]{figures/all_loss_surfaces/DomainNet/TE0_env4_out_loss_plane.pdf}
    \caption{\textit{Real} \scriptsize{(valid)}}
\end{subfigure}
\begin{subfigure}[b]{0.16\columnwidth}
    \includegraphics[width=\textwidth]{figures/all_loss_surfaces/DomainNet/TE0_env5_out_loss_plane.pdf}
    \caption{\textit{Sketch} \scriptsize{(valid)}}
\end{subfigure}
\begin{subfigure}[b]{0.16\columnwidth}
    \includegraphics[width=\textwidth]{figures/all_loss_surfaces/DomainNet/TE0_env0_in_loss_plane.pdf}
    \caption{\textit{Clipart} \scriptsize{(test)}}
\end{subfigure}
\vspace{-0.5em}
\caption{\textbf{Visualization of loss surfaces for \data{DomainNet} when the target domain is \textit{Clipart}.}
}
\label{figure:add_loss_surface_DomainNet_Clipart}
\end{figure}
%%%%%%%%%%%%%%%%%%%%%%%%%%%%%%%%%%%%%%%%%%%%%%%%%%%%%%%%%%%%%%%%%%%%%%%%%%%%%%%%
\begin{figure}[H]
\centering
\captionsetup[subfigure]{aboveskip=0pt,belowskip=0pt}
\begin{subfigure}[b]{0.19\columnwidth}
    \includegraphics[width=\textwidth]{figures/all_loss_surfaces/DomainNet/TE1_env0_in_loss_plane.pdf}
    \caption{\textit{Clipart} \scriptsize{(train)}}
\end{subfigure}
\begin{subfigure}[b]{0.19\columnwidth}
    \includegraphics[width=\textwidth]{figures/all_loss_surfaces/DomainNet/TE1_env2_in_loss_plane.pdf}
    \caption{\textit{Painting} \scriptsize{(train)}}
\end{subfigure}
\begin{subfigure}[b]{0.19\columnwidth}
    \includegraphics[width=\textwidth]{figures/all_loss_surfaces/DomainNet/TE1_env3_in_loss_plane.pdf}
    \caption{\textit{Quickdraw} \scriptsize{(train)}}
\end{subfigure}
\begin{subfigure}[b]{0.19\columnwidth}
    \includegraphics[width=\textwidth]{figures/all_loss_surfaces/DomainNet/TE1_env4_in_loss_plane.pdf}
    \caption{\textit{Real} \scriptsize{(train)}}
\end{subfigure}
\begin{subfigure}[b]{0.19\columnwidth}
    \includegraphics[width=\textwidth]{figures/all_loss_surfaces/DomainNet/TE1_env5_in_loss_plane.pdf}
    \caption{\textit{Sketch} \scriptsize{(train)}}
\end{subfigure}
\\
\begin{subfigure}[b]{0.16\columnwidth}
    \includegraphics[width=\textwidth]{figures/all_loss_surfaces/DomainNet/TE1_env0_out_loss_plane.pdf}
    \caption{\textit{Clipart} \scriptsize{(valid)}}
\end{subfigure}
\begin{subfigure}[b]{0.16\columnwidth}
    \includegraphics[width=\textwidth]{figures/all_loss_surfaces/DomainNet/TE1_env2_out_loss_plane.pdf}
    \caption{\textit{Painting} \scriptsize{(valid)}}
\end{subfigure}
\begin{subfigure}[b]{0.16\columnwidth}
    \includegraphics[width=\textwidth]{figures/all_loss_surfaces/DomainNet/TE1_env3_out_loss_plane.pdf}
    \caption{\textit{Quickdraw} \scriptsize{(valid)}}
\end{subfigure}
\begin{subfigure}[b]{0.16\columnwidth}
    \includegraphics[width=\textwidth]{figures/all_loss_surfaces/DomainNet/TE1_env4_out_loss_plane.pdf}
    \caption{\textit{Real} \scriptsize{(valid)}}
\end{subfigure}
\begin{subfigure}[b]{0.16\columnwidth}
    \includegraphics[width=\textwidth]{figures/all_loss_surfaces/DomainNet/TE1_env5_out_loss_plane.pdf}
    \caption{\textit{Sketch} \scriptsize{(valid)}}
\end{subfigure}
\begin{subfigure}[b]{0.16\columnwidth}
    \includegraphics[width=\textwidth]{figures/all_loss_surfaces/DomainNet/TE1_env1_in_loss_plane.pdf}
    \caption{\textit{Infographic} \scriptsize{(test)}}
\end{subfigure}
\vspace{-0.5em}
\caption{\textbf{Visualization of loss surfaces for \data{DomainNet} when the target domain is \textit{Infographic}.}
}
\label{figure:add_loss_surface_DomainNet_Infographic}
\end{figure}
%%%%%%%%%%%%%%%%%%%%%%%%%%%%%%%%%%%%%%%%%%%%%%%%%%%%%%%%%%%%%%%%%%%%%%%%%%%%%%%%
\begin{figure}[H]
\centering
\captionsetup[subfigure]{aboveskip=0pt,belowskip=0pt}
\begin{subfigure}[b]{0.19\columnwidth}
    \includegraphics[width=\textwidth]{figures/all_loss_surfaces/DomainNet/TE2_env0_in_loss_plane.pdf}
    \caption{\textit{Clipart} \scriptsize{(train)}}
\end{subfigure}
\begin{subfigure}[b]{0.19\columnwidth}
    \includegraphics[width=\textwidth]{figures/all_loss_surfaces/DomainNet/TE2_env1_in_loss_plane.pdf}
    \caption{\textit{Infographic} \scriptsize{(train)}}
\end{subfigure}
\begin{subfigure}[b]{0.19\columnwidth}
    \includegraphics[width=\textwidth]{figures/all_loss_surfaces/DomainNet/TE2_env3_in_loss_plane.pdf}
    \caption{\textit{Quickdraw} \scriptsize{(train)}}
\end{subfigure}
\begin{subfigure}[b]{0.19\columnwidth}
    \includegraphics[width=\textwidth]{figures/all_loss_surfaces/DomainNet/TE2_env4_in_loss_plane.pdf}
    \caption{\textit{Real} \scriptsize{(train)}}
\end{subfigure}
\begin{subfigure}[b]{0.19\columnwidth}
    \includegraphics[width=\textwidth]{figures/all_loss_surfaces/DomainNet/TE2_env5_in_loss_plane.pdf}
    \caption{\textit{Sketch} \scriptsize{(train)}}
\end{subfigure}
\\
\begin{subfigure}[b]{0.16\columnwidth}
    \includegraphics[width=\textwidth]{figures/all_loss_surfaces/DomainNet/TE2_env0_out_loss_plane.pdf}
    \caption{\textit{Clipart} \scriptsize{(valid)}}
\end{subfigure}
\begin{subfigure}[b]{0.16\columnwidth}
    \includegraphics[width=\textwidth]{figures/all_loss_surfaces/DomainNet/TE2_env1_out_loss_plane.pdf}
    \caption{\textit{Infographic} \scriptsize{(valid)}}
\end{subfigure}
\begin{subfigure}[b]{0.16\columnwidth}
    \includegraphics[width=\textwidth]{figures/all_loss_surfaces/DomainNet/TE2_env3_out_loss_plane.pdf}
    \caption{\textit{Quickdraw} \scriptsize{(valid)}}
\end{subfigure}
\begin{subfigure}[b]{0.16\columnwidth}
    \includegraphics[width=\textwidth]{figures/all_loss_surfaces/DomainNet/TE2_env4_out_loss_plane.pdf}
    \caption{\textit{Real} \scriptsize{(valid)}}
\end{subfigure}
\begin{subfigure}[b]{0.16\columnwidth}
    \includegraphics[width=\textwidth]{figures/all_loss_surfaces/DomainNet/TE2_env5_out_loss_plane.pdf}
    \caption{\textit{Sketch} \scriptsize{(valid)}}
\end{subfigure}
\begin{subfigure}[b]{0.16\columnwidth}
    \includegraphics[width=\textwidth]{figures/all_loss_surfaces/DomainNet/TE2_env2_in_loss_plane.pdf}
    \caption{\textit{Painting} \scriptsize{(test)}}
\end{subfigure}
\vspace{-0.5em}
\caption{\textbf{Visualization of loss surfaces for \data{DomainNet} when the target domain is \textit{Painting}.}
}
\label{figure:add_loss_surface_DomainNet_Painting}
\end{figure}
%%%%%%%%%%%%%%%%%%%%%%%%%%%%%%%%%%%%%%%%%%%%%%%%%%%%%%%%%%%%%%%%%%%%%%%%%%%%%%%%
\begin{figure}[H]
\centering
\captionsetup[subfigure]{aboveskip=0pt,belowskip=0pt}
\begin{subfigure}[b]{0.19\columnwidth}
    \includegraphics[width=\textwidth]{figures/all_loss_surfaces/DomainNet/TE3_env0_in_loss_plane.pdf}
    \caption{\textit{Clipart} \scriptsize{(train)}}
\end{subfigure}
\begin{subfigure}[b]{0.19\columnwidth}
    \includegraphics[width=\textwidth]{figures/all_loss_surfaces/DomainNet/TE3_env1_in_loss_plane.pdf}
    \caption{\textit{Infographic} \scriptsize{(train)}}
\end{subfigure}
\begin{subfigure}[b]{0.19\columnwidth}
    \includegraphics[width=\textwidth]{figures/all_loss_surfaces/DomainNet/TE3_env2_in_loss_plane.pdf}
    \caption{\textit{Painting} \scriptsize{(train)}}
\end{subfigure}
\begin{subfigure}[b]{0.19\columnwidth}
    \includegraphics[width=\textwidth]{figures/all_loss_surfaces/DomainNet/TE3_env4_in_loss_plane.pdf}
    \caption{\textit{Real} \scriptsize{(train)}}
\end{subfigure}
\begin{subfigure}[b]{0.19\columnwidth}
    \includegraphics[width=\textwidth]{figures/all_loss_surfaces/DomainNet/TE3_env5_in_loss_plane.pdf}
    \caption{\textit{Sketch} \scriptsize{(train)}}
\end{subfigure}
\\
\begin{subfigure}[b]{0.16\columnwidth}
    \includegraphics[width=\textwidth]{figures/all_loss_surfaces/DomainNet/TE3_env0_out_loss_plane.pdf}
    \caption{\textit{Clipart} \scriptsize{(valid)}}
\end{subfigure}
\begin{subfigure}[b]{0.16\columnwidth}
    \includegraphics[width=\textwidth]{figures/all_loss_surfaces/DomainNet/TE3_env1_out_loss_plane.pdf}
    \caption{\textit{Infographic} \scriptsize{(valid)}}
\end{subfigure}
\begin{subfigure}[b]{0.16\columnwidth}
    \includegraphics[width=\textwidth]{figures/all_loss_surfaces/DomainNet/TE3_env2_out_loss_plane.pdf}
    \caption{\textit{Painting} \scriptsize{(valid)}}
\end{subfigure}
\begin{subfigure}[b]{0.16\columnwidth}
    \includegraphics[width=\textwidth]{figures/all_loss_surfaces/DomainNet/TE3_env4_out_loss_plane.pdf}
    \caption{\textit{Real} \scriptsize{(valid)}}
\end{subfigure}
\begin{subfigure}[b]{0.16\columnwidth}
    \includegraphics[width=\textwidth]{figures/all_loss_surfaces/DomainNet/TE3_env5_out_loss_plane.pdf}
    \caption{\textit{Sketch} \scriptsize{(valid)}}
\end{subfigure}
\begin{subfigure}[b]{0.16\columnwidth}
    \includegraphics[width=\textwidth]{figures/all_loss_surfaces/DomainNet/TE3_env3_in_loss_plane.pdf}
    \caption{\textit{Quickdraw} \scriptsize{(test)}}
\end{subfigure}
\vspace{-0.5em}
\caption{\textbf{Visualization of loss surfaces for \data{DomainNet} when the target domain is \textit{Quickdraw}.}
}
\label{figure:add_loss_surface_DomainNet_Quickdraw}
\end{figure}
%%%%%%%%%%%%%%%%%%%%%%%%%%%%%%%%%%%%%%%%%%%%%%%%%%%%%%%%%%%%%%%%%%%%%%%%%%%%%%%%
\begin{figure}[H]
\centering
\captionsetup[subfigure]{aboveskip=0pt,belowskip=0pt}
\begin{subfigure}[b]{0.19\columnwidth}
    \includegraphics[width=\textwidth]{figures/all_loss_surfaces/DomainNet/TE4_env0_in_loss_plane.pdf}
    \caption{\textit{Clipart} \scriptsize{(train)}}
\end{subfigure}
\begin{subfigure}[b]{0.19\columnwidth}
    \includegraphics[width=\textwidth]{figures/all_loss_surfaces/DomainNet/TE4_env1_in_loss_plane.pdf}
    \caption{\textit{Infographic} \scriptsize{(train)}}
\end{subfigure}
\begin{subfigure}[b]{0.19\columnwidth}
    \includegraphics[width=\textwidth]{figures/all_loss_surfaces/DomainNet/TE4_env2_in_loss_plane.pdf}
    \caption{\textit{Painting} \scriptsize{(train)}}
\end{subfigure}
\begin{subfigure}[b]{0.19\columnwidth}
    \includegraphics[width=\textwidth]{figures/all_loss_surfaces/DomainNet/TE4_env3_in_loss_plane.pdf}
    \caption{\textit{Quickdraw} \scriptsize{(train)}}
\end{subfigure}
\begin{subfigure}[b]{0.19\columnwidth}
    \includegraphics[width=\textwidth]{figures/all_loss_surfaces/DomainNet/TE4_env5_in_loss_plane.pdf}
    \caption{\textit{Sketch} \scriptsize{(train)}}
\end{subfigure}
\\
\begin{subfigure}[b]{0.16\columnwidth}
    \includegraphics[width=\textwidth]{figures/all_loss_surfaces/DomainNet/TE4_env0_out_loss_plane.pdf}
    \caption{\textit{Clipart} \scriptsize{(valid)}}
\end{subfigure}
\begin{subfigure}[b]{0.16\columnwidth}
    \includegraphics[width=\textwidth]{figures/all_loss_surfaces/DomainNet/TE4_env1_out_loss_plane.pdf}
    \caption{\textit{Infographic} \scriptsize{(valid)}}
\end{subfigure}
\begin{subfigure}[b]{0.16\columnwidth}
    \includegraphics[width=\textwidth]{figures/all_loss_surfaces/DomainNet/TE4_env2_out_loss_plane.pdf}
    \caption{\textit{Painting} \scriptsize{(valid)}}
\end{subfigure}
\begin{subfigure}[b]{0.16\columnwidth}
    \includegraphics[width=\textwidth]{figures/all_loss_surfaces/DomainNet/TE4_env3_out_loss_plane.pdf}
    \caption{\textit{Quickdraw} \scriptsize{(valid)}}
\end{subfigure}
\begin{subfigure}[b]{0.16\columnwidth}
    \includegraphics[width=\textwidth]{figures/all_loss_surfaces/DomainNet/TE4_env5_out_loss_plane.pdf}
    \caption{\textit{Sketch} \scriptsize{(valid)}}
\end{subfigure}
\begin{subfigure}[b]{0.16\columnwidth}
    \includegraphics[width=\textwidth]{figures/all_loss_surfaces/DomainNet/TE4_env4_in_loss_plane.pdf}
    \caption{\textit{Real} \scriptsize{(test)}}
\end{subfigure}
\vspace{-0.5em}
\caption{\textbf{Visualization of loss surfaces for \data{DomainNet} when the target domain is \textit{Real}.}
}
\label{figure:add_loss_surface_DomainNet_Real}
\end{figure}
%%%%%%%%%%%%%%%%%%%%%%%%%%%%%%%%%%%%%%%%%%%%%%%%%%%%%%%%%%%%%%%%%%%%%%%%%%%%%%%%
\begin{figure}[H]
\centering
\captionsetup[subfigure]{aboveskip=0pt,belowskip=0pt}
\begin{subfigure}[b]{0.19\columnwidth}
    \includegraphics[width=\textwidth]{figures/all_loss_surfaces/DomainNet/TE5_env0_in_loss_plane.pdf}
    \caption{\textit{Clipart} \scriptsize{(train)}}
\end{subfigure}
\begin{subfigure}[b]{0.19\columnwidth}
    \includegraphics[width=\textwidth]{figures/all_loss_surfaces/DomainNet/TE5_env1_in_loss_plane.pdf}
    \caption{\textit{Infographic} \scriptsize{(train)}}
\end{subfigure}
\begin{subfigure}[b]{0.19\columnwidth}
    \includegraphics[width=\textwidth]{figures/all_loss_surfaces/DomainNet/TE5_env2_in_loss_plane.pdf}
    \caption{\textit{Painting} \scriptsize{(train)}}
\end{subfigure}
\begin{subfigure}[b]{0.19\columnwidth}
    \includegraphics[width=\textwidth]{figures/all_loss_surfaces/DomainNet/TE5_env3_in_loss_plane.pdf}
    \caption{\textit{Quickdraw} \scriptsize{(train)}}
\end{subfigure}
\begin{subfigure}[b]{0.19\columnwidth}
    \includegraphics[width=\textwidth]{figures/all_loss_surfaces/DomainNet/TE5_env4_in_loss_plane.pdf}
    \caption{\textit{Real} \scriptsize{(train)}}
\end{subfigure}
\\
\begin{subfigure}[b]{0.16\columnwidth}
    \includegraphics[width=\textwidth]{figures/all_loss_surfaces/DomainNet/TE5_env0_out_loss_plane.pdf}
    \caption{\textit{Clipart} \scriptsize{(valid)}}
\end{subfigure}
\begin{subfigure}[b]{0.16\columnwidth}
    \includegraphics[width=\textwidth]{figures/all_loss_surfaces/DomainNet/TE5_env1_out_loss_plane.pdf}
    \caption{\textit{Infographic} \scriptsize{(valid)}}
\end{subfigure}
\begin{subfigure}[b]{0.16\columnwidth}
    \includegraphics[width=\textwidth]{figures/all_loss_surfaces/DomainNet/TE5_env2_out_loss_plane.pdf}
    \caption{\textit{Painting} \scriptsize{(valid)}}
\end{subfigure}
\begin{subfigure}[b]{0.16\columnwidth}
    \includegraphics[width=\textwidth]{figures/all_loss_surfaces/DomainNet/TE5_env3_out_loss_plane.pdf}
    \caption{\textit{Quickdraw} \scriptsize{(valid)}}
\end{subfigure}
\begin{subfigure}[b]{0.16\columnwidth}
    \includegraphics[width=\textwidth]{figures/all_loss_surfaces/DomainNet/TE5_env4_out_loss_plane.pdf}
    \caption{\textit{Real} \scriptsize{(valid)}}
\end{subfigure}
\begin{subfigure}[b]{0.16\columnwidth}
    \includegraphics[width=\textwidth]{figures/all_loss_surfaces/DomainNet/TE5_env5_in_loss_plane.pdf}
    \caption{\textit{Sketch} \scriptsize{(test)}}
\end{subfigure}
\vspace{-0.5em}
\caption{\textbf{Visualization of loss surfaces for \data{DomainNet} when the target domain is \textit{Sketch}.}
}
\label{figure:add_loss_surface_DomainNet_Sketch}
\end{figure}
%%%%%%%%%%%%%%%%%%%%%%%%%%%%%%%%%%%%%%%%%%%%%%%%%%%%%%%%%%%%%%%%%%%%%%%%%%%%%%%%
